# Supplementary material for: Reduced Robust Random Cut Forest for Out-Of-Distribution detection in machine learning models
Source: arXiv:2206.09247 source file (2022-06-18)
Supplement: Supplementary file 1 [file Appendix.tex]

\section{Appendix I}
\setlength{\parskip}{0pt}
\setlength{\parsep}{0pt}
\setlength{\headsep}{0pt}
\setlength{\topskip}{0pt}
\setlength{\topmargin}{0pt}
\setlength{\topsep}{0pt}
\setlength{\partopsep}{0pt}
\captionsetup{justification=raggedright,singlelinecheck=false}
\label{sec:appendix}

\begin{algorithm}
\SetKwInOut{Input}{Input}
\SetKwInOut{Output}{Output}
\SetAlgoLined
\caption{CreateTree()}
\label{alg:createtree}
\Input{Data $Y$ of size $n$, each having dimension $d$}
\Output{A Robust Random Cut Tree $T(Y)$ }

 \While{Size(Y_i) != 0}{
   $r_i= max_{X \in Y}(X_i)-min_{X \in Y}(X_i) \;\forall i\in d $\\
   $p_i= \dfrac{r_i}{\sum_{i=1}^{i=d}r_i} \;\forall i$ \\
   $k= random(0-1)$ \\
   map k on $p_i$ and select corresponding dimension \\
   $choose \; X_i \mid X_i \in Uniform(max(X_i)-min(X_i)) \forall X \in Y$ \\
   $Y_1={X_i} $\\
   $Y_2= Y \setminus Y_1$ \\
 }
\end{algorithm}

\begin{algorithm}
\SetKwInOut{Input}{Input}
\SetKwInOut{Output}{Output}
\SetKwInOut{Parameter}{parameter}
\SetAlgoLined
\caption{CreateForest()}
\label{alg:createforest}
\Input{Data Y}
\Output{Robust Random Cut forest }
\Parameter{number of trees in forest}
 initialization: forest=[ ]\;
 \While{(length of forest) \leq number of trees}
 {
   tree=CreateTree(Y) \; 
   forest.append(tree)
 }
\end{algorithm}

\begin{algorithm}
\SetKwInOut{Input}{Input}
\SetKwInOut{Output}{Output}
\SetKwInOut{Parameter}{parameter}
\SetAlgoLined
\caption{Deletepoint()}
\label{alg:deletepoint}
\Input{tree $T(Y)$ and point $x \in Y$}
\Output{tree $T(Y - x$) }

 find leaf corresponding to point $x$ in $T$ \\
 find sibling node of $x$, assume its $a$ \\
 delete the parent node of $x$ and replace it by $a$
\end{algorithm}

\begin{algorithm}
\SetKwInOut{Input}{Input}
\SetKwInOut{Output}{Output}
\SetKwInOut{Parameter}{parameter}
\SetAlgoLined
\caption{Insertpoint()}
\label{alg:insertpoint}
\Input{tree $T(Y) $ and data-point $x \mid x \notin Y$}
\Output{tree $T(Y \cup x$) }
 initialization\;
 \While{While condition}{
  instructions\;
  \eIf{condition}{
   instructions1\;
   instructions2\;
   }{
   instructions3\;
  }
 }
\end{algorithm}
